# Supplementary material for: On the uncertainty principle of neural networks
Source: arXiv:2205.01493 source file (2025-01-16)
Supplement: Supplementary file 1 [file sn-articlesi.tex]

\documentclass[10pt,journal,compsoc,onecolumn]{IEEEtran}
%
% If IEEEtran.cls has not been installed into the LaTeX system files,
% manually specify the path to it like:
% \documentclass[10pt,journal,compsoc]{../sty/IEEEtran}
\usepackage[T1]{fontenc}
\usepackage[utf8]{inputenc}
\usepackage{babel}
\usepackage{pifont}
\usepackage{pmboxdraw}
\usepackage{amsmath}
\usepackage{amssymb}
\usepackage{graphicx}
\usepackage{wasysym}
\usepackage{booktabs}
\usepackage{multirow}
\usepackage{amsthm}
\newtheorem{theorem}{Theorem}

\usepackage{makecell}
\providecommand{\tabularnewline}{\\}

% Some very useful LaTeX packages include:
% (uncomment the ones you want to load)

% *** MISC UTILITY PACKAGES ***
%
%\usepackage{ifpdf}
% Heiko Oberdiek's ifpdf.sty is very useful if you need conditional
% compilation based on whether the output is pdf or dvi.
% usage:
% \ifpdf
%   % pdf code
% \else
%   % dvi code
% \fi
% The latest version of ifpdf.sty can be obtained from:
% http://www.ctan.org/pkg/ifpdf
% Also, note that IEEEtran.cls V1.7 and later provides a builtin
% \ifCLASSINFOpdf conditional that works the same way.
% When switching from latex to pdflatex and vice-versa, the compiler may
% have to be run twice to clear warning/error messages.

% *** CITATION PACKAGES ***
%
\ifCLASSOPTIONcompsoc
  % IEEE Computer Society needs nocompress option
  % requires cite.sty v4.0 or later (November 2003)
  \usepackage[nocompress]{cite}
\else
  % normal IEEE
  \usepackage{cite}
\fi
% cite.sty was written by Donald Arseneau
% V1.6 and later of IEEEtran pre-defines the format of the cite.sty package
% \cite{} output to follow that of the IEEE. Loading the cite package will
% result in citation numbers being automatically sorted and properly
% "compressed/ranged". e.g., [1], [9], [2], [7], [5], [6] without using
% cite.sty will become [1], [2], [5]--[7], [9] using cite.sty. cite.sty's
% \cite will automatically add leading space, if needed. Use cite.sty's
% noadjust option (cite.sty V3.8 and later) if you want to turn this off
% such as if a citation ever needs to be enclosed in parenthesis.
% cite.sty is already installed on most LaTeX systems. Be sure and use
% version 5.0 (2009-03-20) and later if using hyperref.sty.
% The latest version can be obtained at:
% http://www.ctan.org/pkg/cite
% The documentation is contained in the cite.sty file itself.
%
% Note that some packages require special options to format as the Computer
% Society requires. In particular, Computer Society  papers do not use
% compressed citation ranges as is done in typical IEEE papers
% (e.g., [1]-[4]). Instead, they list every citation separately in order
% (e.g., [1], [2], [3], [4]). To get the latter we need to load the cite
% package with the nocompress option which is supported by cite.sty v4.0
% and later. Note also the use of a CLASSOPTION conditional provided by
% IEEEtran.cls V1.7 and later.

% *** GRAPHICS RELATED PACKAGES ***
%
\ifCLASSINFOpdf
  % \usepackage[pdftex]{graphicx}
  % declare the path(s) where your graphic files are
  % \graphicspath{{../pdf/}{../jpeg/}}
  % and their extensions so you won't have to specify these with
  % every instance of \includegraphics
  % \DeclareGraphicsExtensions{.pdf,.jpeg,.png}
\else
  % or other class option (dvipsone, dvipdf, if not using dvips). graphicx
  % will default to the driver specified in the system graphics.cfg if no
  % driver is specified.
  % \usepackage[dvips]{graphicx}
  % declare the path(s) where your graphic files are
  % \graphicspath{{../eps/}}
  % and their extensions so you won't have to specify these with
  % every instance of \includegraphics
  % \DeclareGraphicsExtensions{.eps}
\fi
\hyphenation{op-tical net-works semi-conduc-tor}

\begin{document}

\newcommand{\tabincell}[2]
{\begin{tabular}
{@{}#1@{}}#2\end{tabular}}
%
% paper title
% Titles are generally capitalized except for words such as a, an, and, as,
% at, but, by, for, in, nor, of, on, or, the, to and up, which are usually
% not capitalized unless they are the first or last word of the title.
% Linebreaks \\ can be used within to get better formatting as desired.
% Do not put math or special symbols in the title.
\title{On The Uncertainty Principle of Neural Networks: Supplementary Information}
%
%
% author names and IEEE memberships
% note positions of commas and nonbreaking spaces ( ~ ) LaTeX will not break
% a structure at a ~ so this keeps an author's name from being broken across
% two lines.
% use \thanks{} to gain access to the first footnote area
% a separate \thanks must be used for each paragraph as LaTeX2e's \thanks
% was not built to handle multiple paragraphs
%
%
%\IEEEcompsocitemizethanks is a special \thanks that produces the bulleted
% lists the Computer Society journals use for "first footnote" author
% affiliations. Use \IEEEcompsocthanksitem which works much like \item
% for each affiliation group. When not in compsoc mode,
% \IEEEcompsocitemizethanks becomes like \thanks and
% \IEEEcompsocthanksitem becomes a line break with idention. This
% facilitates dual compilation, although admittedly the differences in the
% desired content of \author between the different types of papers makes a
% one-size-fits-all approach a daunting prospect. For instance, compsoc
% journal papers have the author affiliations above the "Manuscript
% received ..."  text while in non-compsoc journals this is reversed. Sigh.

\author{Jun-Jie Zhang,
        Dong-Xiao Zhang,
        Jian-Nan Chen,
        Long-Gang Pang,
        and Deyu Meng % <-this % stops a space
\IEEEcompsocitemizethanks{\IEEEcompsocthanksitem J.-J. Zhang, D.-X. Zhang and J.-N. Chen are with the Division of Computational physics and Intelligent modeling, Northwest
Institute of Nuclear Technology, Shaanxi, Xi’an 710024, China\protect\\
% note need leading \protect in front of \\ to get a newline within \thanks as
% \\ is fragile and will error, could use \hfil\break instead.
E-mail: zjacob@mail.ustc.edu.cn
\IEEEcompsocthanksitem L.-G. Pang is with the Key Laboratory of Quark \& Lepton Physics of Ministry of Education,
Central China Normal University, Wuhan 430079, China.% <-this % stops an unwanted space
\IEEEcompsocthanksitem D. Meng is with School of Mathematics and Statistics and Ministry of Education Key Lab of Intelligent Networks and Network Security,
Xi'an Jiaotong University, Shaanxi, P. R. China.\\
Email: dymeng@mail.xjtu.edu.cn}% <-this % stops an unwanted space
}

\IEEEtitleabstractindextext{%
\begin{abstract}
In this supplementary material, we provide some background information of the FGSM attack and uncertainty principle in physics. Then we derive the uncertainty principle for neural networks in detail.

\end{abstract}
}

% make the title area
\maketitle

% To allow for easy dual compilation without having to reenter the
% abstract/keywords data, the \IEEEtitleabstractindextext text will
% not be used in maketitle, but will appear (i.e., to be "transported")
% here as \IEEEdisplaynontitleabstractindextext when the compsoc
% or transmag modes are not selected <OR> if conference mode is selected
% - because all conference papers position the abstract like regular
% papers do.
\IEEEdisplaynontitleabstractindextext
% \IEEEdisplaynontitleabstractindextext has no effect when using
% compsoc or transmag under a non-conference mode.

% For peer review papers, you can put extra information on the cover
% page as needed:
% \ifCLASSOPTIONpeerreview
% \begin{center} \bfseries EDICS Category: 3-BBND \end{center}
% \fi
%
% For peerreview papers, this IEEEtran command inserts a page break and
% creates the second title. It will be ignored for other modes.
\IEEEpeerreviewmaketitle

\section*{Some background information}

\subsection*{The FGSM attack}

One of the most classical and simplest attacking methods is the Fast Gradient
Sign Method\cite{goodfellow2015explaining} (FGSM) presented by Goodfellow et al. in 2015. Given a loss function $l(f(X,\theta),Y^{*})$, the
FGSM creates an attack $X$ by
\begin{eqnarray}
X & = & X_{0}+\epsilon\cdot\text{sign}(\nabla_{X}l(f(X,\theta),Y^{*})| _{X=X_0}),\label{eq:FGSM1}
\end{eqnarray}
where the loss function $l$ is obtained under a network model $f(X,\theta)$ with parameters $\theta$ trained on a pre-collected training dataset, and $\epsilon$ is a positive number usually taken to be a small value to make the attack possibly imperceptible. $X_{0}$ denotes the raw image to be attacked and classified, and $Y^{*}$
is the true label for image $X_{0}$. Here, $\nabla_{X}l(f(X,\theta),Y^{*})$
is interpreted as the gradient of $l$ with respect to $X$. For most of the classifiers, the loss function $l$ is simply the training loss used in training the network. Note that the choice of the loss function does not significantly affect the performance of the attack \cite{10.1007/978-3-031-06767-9_17,ijcai2021p635}.
Since the gradient is not difficult to compute for deep neural networks, the attack can always be efficiently implemented.

\subsection*{Uncertainty principle in quantum physics}

In this subsection, all physical quantities are expressed in the natural unit.
In quantum physics, we can describe a particle by a wave packet $\psi(X)$
in the coordinate representation with respect to the coordinate reference
frame. The normailzation condition for $\psi(X)$ is given by
\begin{eqnarray}
\int|\psi(X)|^{2}dX & = & 1,\label{eq:normalization}
\end{eqnarray}
where the square amplitude $|\psi(X)|^{2}$ gives the probability
density for finding a particle at position $X=(x,y,z)$. To measure the physical
quantities of the particle, such as position $X$ and momentum $P=(p_{x},p_{y},p_{z})$,
we need to define the position and momentum operators $\hat{x}_{i}$
and $\hat{p}_{i}$ as:
\begin{eqnarray}
\hat{x}_{i}\psi(X) & = & x_{i}\psi(X),\nonumber \\
\hat{p}_{i}\psi(X) & = & -i\frac{\partial}{\partial x_{i}}\psi(X),\label{eq:operators}
\end{eqnarray}
where $i=1,2,3$ denote the $x,y,z$ components in the coordinate
space, respectively. The
average position and momentum of the particle can be evaluated by
\begin{eqnarray}
\langle\hat{x}_{i}\rangle & = & \int\psi^{*}(X)x_{i}\psi(X)dX\nonumber \\
\langle\hat{p}_{i}\rangle & = & \int\psi^{*}(X)[-i\frac{\partial}{\partial x_{i}}\psi(X)]dX,\label{eq:average_values}
\end{eqnarray}
where $\langle\cdot\rangle$ is the Dirac symbol widely used in physics
and $\psi^{*}(X)$ is the complex conjugate of $\psi(X)$.
The standard deviations of the position $\sigma_{x_{i}}$ and momentum
$\sigma_{p_{i}}$ are defined respectively as:
\begin{eqnarray}
\sigma_{x_{i}} & = & \langle(\hat{x}_{i}-\langle\hat{x}_{i}\rangle)^{2}\rangle^{1/2},\nonumber \\
\sigma_{p_{i}} & = & \langle(\hat{p}_{i}-\langle\hat{p}_{i}\rangle)^{2}\rangle^{1/2}.\label{eq:sigma_qu}
\end{eqnarray}

In the year of 1927, Heisenberg introduced the first formulation of the
uncertainty principle in his German article\cite{Heisenberg1927}.
The Heisenberg's uncertainty principle asserts a fundamental limit
to the accuracy for certain pairs. Such variable pairs are known as complementary variables (or
canonically conjugate variables). The formal inequality relating the
standard deviation of position $\sigma_{x_{i}}$ and the standard
deviation of momentum $\sigma_{p_{i}}$ reads
\begin{eqnarray}
\sigma_{x_{i}}\sigma_{p_{i}} & \geq & \frac{1}{2}.\label{eq:Un_re_Qu}
\end{eqnarray}
Uncertainty relation Eq. (\ref{eq:Un_re_Qu}) states a fundamental
property of quantum systems and can be understood in terms of the Niels
Bohr\textquoteright s complementarity principle\cite{Bohr1950}. That is, objects have certain pairs of complementary properties cannot
be observed or measured simultaneously.

\section*{Uncertainty principle for neural networks}

\subsection*{Neural Network Notation and Loss Function Integration}

For the purpose of this study, we proceed with the assumption that the loss function $l(f(X,\theta),Y)$, representing the discrepancy between the neural network's prediction and the actual output, is square integrable. This is a reasonable assumption in practice, as outlier samples with loss values exceeding a certain threshold $C$ are typically discounted as irrelevant to the problem at hand. Such a constraint ensures that the loss function remains square integrable within the functional range of interest.

We express this requirement mathematically as: \begin{eqnarray} \int l(f(X,\theta),Y)^{2}dX & = & \beta.\label{eq:normalize_ne} \end{eqnarray} Normalization of the loss function is achieved by dividing by the square root of $\beta$, resulting in a new function $\psi_{Y}(X)$: \begin{eqnarray} \psi_{Y}(X) & = & \frac{l(f(X,\theta),Y)}{\beta^{1/2}},\label{eq:L} \end{eqnarray} which satisfies the condition: \begin{eqnarray} \int \psi_{Y}(X)^{2}dX=1.\label{eq:} \end{eqnarray} For the purposes of our analysis, we refer to $\psi_{Y}(X)$ as a 'neural packet', a term that encapsulates the distribution of prediction errors across the input space. Each label $Y$ corresponds to a distinct neural packet, reflecting the network's performance on different classes of inputs.

To facilitate our analysis, we conceptualize an image $X = (x_{1}, ..., x_{i}, ..., x_{M})$ with $M$ pixels as a point in a multidimensional space, with the pixel values represented numerically by the vector components. In this framework, we define the pixel and attack operators for a neural packet $\psi_{Y}(X)$ as follows: 
\begin{eqnarray}
\hat{x}_{i}\psi_{Y}(X) & = & x_{i}\psi_{Y}(X),\nonumber \\
\hat{p}_{i}\psi_{Y}(X) & = & \frac{\partial}{\partial x_{i}}\psi_{Y}(X).\label{eq:operator_nu}
\end{eqnarray}
The average pixel value at position $x_{i}$ associated with the neural packet can be computed using the operator $\hat{x}_{i}$: 
\begin{eqnarray} \langle\hat{x}_{i}\rangle & = & \int \psi_{Y}(X)x_{i}\psi_{Y}(X)dX.\label{eq:ave_x_nu} \end{eqnarray} 

As we are working with real-valued functions, the complex conjugate is not needed in this context.

Furthermore, the attack operator $\hat{p}_{i} = \frac{\partial}{\partial x{i}}$ represents the conjugate variable to pixel value $x_{i}$. The average attack effect can be determined as the expectation value of $\hat{p}_{i}$: 

\begin{eqnarray} \langle\hat{p}_{i}\rangle & = & \int \psi_{Y}(X)\frac{\partial}{\partial x_{i}}\psi_{Y}(X)dX.\label{eq:ave_p_nu} \end{eqnarray}

\subsection*{Derivation of the uncertainty relation}\label{sec:direvation-detail}

\begin{table*}
\centering
\caption{Comparison of the uncertainty principle between quantum physics and neural networks.\label{tab:Comparison-of-the uncertainty}}
\resizebox{\linewidth}{!}{
\begin{tabular}{cc|cc}
\toprule
\multicolumn{2}{c}{Quantum physics} & \multicolumn{2}{c}{Neural networks}\tabularnewline
\midrule
position & $X=(x,y,z)$ & $X=(x_{1},...,x_{i},...,x_{M})$ & image (input)\tabularnewline
\midrule
\tabincell{c}{momentum \\ (conjugate of position)} & $P=(p_{x},p_{y},p_{z})$ & $P=(p_{1},...,p_{i},...,p_{M})$ & \tabincell{c}{attack \\(conjugate of input)}\tabularnewline
\midrule
wave function & $\psi(X)$ & $\psi_{Y}(X)$ & \tabincell{c}{normalized loss function \\(neural packet)}\tabularnewline
\midrule
normalize condition & $\int|\psi(X)|^{2}dX=1$ & $\int|\psi_{Y}(X)|^{2}=1$ & normalize condition\tabularnewline
\midrule
position operator & $\hat{x}_{i}\psi(X)=x_{i}\psi(X)$ & $\hat{x}_{i}\psi_{Y}(X)=x_{i}\psi_{Y}(X)$ & pixel operator\tabularnewline
\midrule
momentum operator & $\hat{p}_{i}\psi(X)=-i\frac{\partial}{\partial x_{i}}\psi(X)$ & $\hat{p}_{i}\psi_{Y}(X)=\frac{\partial}{\partial x_{i}}\psi_{Y}(X)$ & attack operator\tabularnewline
\midrule
\tabincell{c}{standard deviation for \\ measuring position} & $\sigma_{x_{i}}=\langle(\hat{x}_{i}-\langle\hat{x}_{i}\rangle)^{2}\rangle^{1/2}$ & $\sigma_{x_{i}}=\langle(\hat{x}_{i}-\langle\hat{x}_{i}\rangle)^{2}\rangle^{1/2}$ & \tabincell{c}{standard deviation for \\ resolving pixel}\tabularnewline
\midrule
\tabincell{c}{standard deviation for \\ measuring momentum} & $\sigma_{p_{i}}=\langle(\hat{p}_{i}-\langle\hat{p}_{i}\rangle)^{2}\rangle^{1/2}$ & $\sigma_{p_{i}}=\langle(\hat{p}_{i}-\langle\hat{p}_{i}\rangle)^{2}\rangle^{1/2}$ & \tabincell{c}{standard deviation for \\ resolving attack}\tabularnewline
\midrule
uncertainty relation & $\sigma_{x_{i}}\sigma_{p_{i}}\geq\frac{1}{2}$ & $\sigma_{x_{i}}\sigma_{p_{i}}\geq\frac{1}{2}$ & uncertainty relation\tabularnewline
\bottomrule
\end{tabular}}
\end{table*}

The uncertainty principle of a trained neural network can then be deduced by the following theorem:
\begin{theorem} The standard deviations $\sigma_{{p}_{i}}$ and $\sigma_{{x}_{i}}$ corresponding to the attack and pixel operators $\hat{p_{i}}$ and $\hat{x_{i}}$, respectively, are restricted by the relation:
\begin{eqnarray}
\sigma_{{p}_{i}}\sigma_{{x}_{i}} & \geq & \frac{1}{2}.
\end{eqnarray}
\end{theorem}
\begin{proof}
We first introduce the standard deviations $\sigma_{a}$ and $\sigma_{b}$
corresponding to two general operators $\hat{A}$ and \textbf{$\hat{B}$}. Then it follows that:
\begin{eqnarray}
\sigma_{a}\sigma_{b} = \langle(\hat{A}-\langle\hat{A}\rangle)^{2}\rangle^{\frac{1}{2}}\langle(\hat{B}-\langle\hat{B}\rangle)^{2}\rangle^{\frac{1}{2}} \equiv \langle\hat{a}^{2}\rangle^{\frac{1}{2}}\langle\hat{b}^{2}\rangle^{\frac{1}{2}}.\nonumber \\
\label{eq:sasb}
\end{eqnarray}
In general, for any two unbounded real operators $\langle\hat{a}\rangle$
and \textbf{$\langle\hat{b}\rangle$}, the following relation holds
\begin{eqnarray}
0\le\langle(\hat{a}-i\hat{b})^{2}\rangle = \langle\hat{a}^{2}\rangle-i\langle\hat{a}\hat{b}-\hat{b}\hat{a}\rangle+\langle\hat{b}^{2}\rangle.\nonumber \\
\label{eq:prove1}
\end{eqnarray}
If we further replace $\hat{a}$ and $\hat{b}$ in Eq. (\ref{eq:prove1}) by operators $\hat{a}\langle\hat{a}^{2}\rangle^{-1/2}$ and $\hat{b}\langle\hat{b}^{2}\rangle^{-1/2}$, we can then obtain the property $2\langle\hat{a}^{2}\rangle^{1/2}\langle\hat{b}^{2}\rangle{}^{1/2} \geq i\langle\hat{a}\hat{b}-\hat{b}\hat{a}\rangle$,
which gives the basic bound for the commutator $[\hat{a},\hat{b}]\equiv\hat{a}\hat{b}-\hat{b}\hat{a}$,
\begin{eqnarray}
\langle\hat{a}^{2}\rangle^{\frac{1}{2}}\langle\hat{b}^{2}\rangle^{\frac{1}{2}} & \geq & |i\frac{1}{2}\langle[\hat{a},\hat{b}]\rangle|.\label{eq:general_uncertainty}
\end{eqnarray}
Seeing the fact that $[\hat{a},\hat{b}]=[\hat{A},\hat{B}]$, we finally obtain the uncertainty relation
\begin{eqnarray}
\sigma_{a}\sigma_{b} & \geq & |i\frac{1}{2}\langle[\hat{A},\hat{B}]\rangle|.\label{eq:general_uncertainty2}
\end{eqnarray}

In terms of the neural networks, we can simply replace operators $\hat{A}$
and $\hat{B}$ by $\hat{p}_{i}$ and $\hat{x}_{i}$ introduced in
Eq. (\ref{eq:operator_nu}), and this leads
to
\begin{eqnarray}
\sigma_{{p}_{i}}\sigma_{{x}_{i}} & \geq & |i\frac{1}{2}\langle[\hat{p}_{i},\hat{x}_{i}]\rangle| = \frac{1}{2},\label{eq:uncertainty_relation}
\end{eqnarray}
where we have used the relation
\begin{eqnarray}
[\hat{p}_{i},\hat{x}_{i}]\psi_{Y}(X) & = & [\hat{p}_{i}\hat{x}_{i}-\hat{x}_{i}\hat{p}_{i}]\psi_{Y}(X)\nonumber \\
& = & \frac{\partial}{\partial x_{i}}[x_{i}\psi_{Y}(X)] \nonumber \\
& & -x_{i}\frac{\partial}{\partial x_{i}}\psi_{Y}(X)\nonumber \\
 & = & \psi_{Y}(X).\label{eq:eigencommutator}
\end{eqnarray}
\end{proof}

Note that for a trained neural network, $\psi_{Y}(X)$ depends on the dataset and the structure of the network.

Eq. (\ref{eq:uncertainty_relation}) is a general result
for general neural networks (see extension to the generation network in supplementary material). For convenience, we compare the formulas in quantum physics with
those used in neural networks in Tab. \ref{tab:Comparison-of-the uncertainty} to facilitate easy understandings for readers.

In the FGSM attack, the attacked image is of the form:
\begin{eqnarray}
X & = & X_{0}+\epsilon\cdot\text{sign}(\nabla_{X}l(f(X,\theta),Y^{*})| _{X=X_0})\nonumber \\
 & \sim & X_{0}+\epsilon\cdot\nabla_{X}l(f(X,\theta),Y^{*})| _{X=X_0}\nonumber \\
 & = & X_{0}+\epsilon\cdot\nabla_{X}[\beta^{1/2}\psi_{Y^*}(X_0)]\nonumber \\
 & = & X_{0}+\epsilon^{\prime}\hat{P}\psi_{Y^*}(X_0),\label{eq:attack_X}
\end{eqnarray}
where $\hat{P}=(\frac{\partial}{\partial x_{1}},...,\frac{\partial}{\partial x_{i}},...,\frac{\partial}{\partial x_{M}})$
and $\epsilon^{\prime}=\epsilon\cdot\beta^{1/2}$. In the second
line of Eq. (\ref{eq:attack_X}) we have used the property substantiated in \cite{agarwal2020the}: ''even
without the 'Sign' of the FGSM, a successful attack can also be achieved". From Eq. (\ref{eq:attack_X}), we can then obtain
\begin{eqnarray}
\hat{P}\psi_{Y^*}(X_0)  \sim \epsilon/\epsilon^{\prime}\cdot\text{sign}(\nabla_{X}l(f(X,\theta),Y^{*})| _{X=X_0}),\label{eq:definition_attack}
\end{eqnarray}
which is the reason that we call $\hat{p_{i}}$ the attack operator.

\subsection*{The frequency-principle explanation}

\begin{figure}
\includegraphics[scale=0.5]{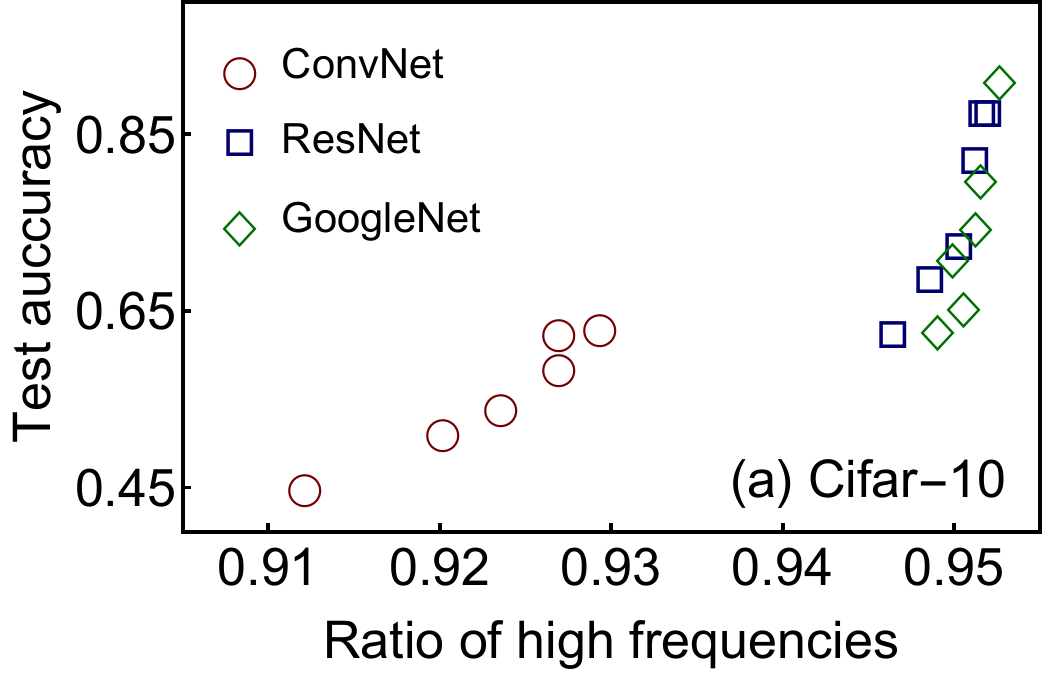}
\includegraphics[scale=0.5]{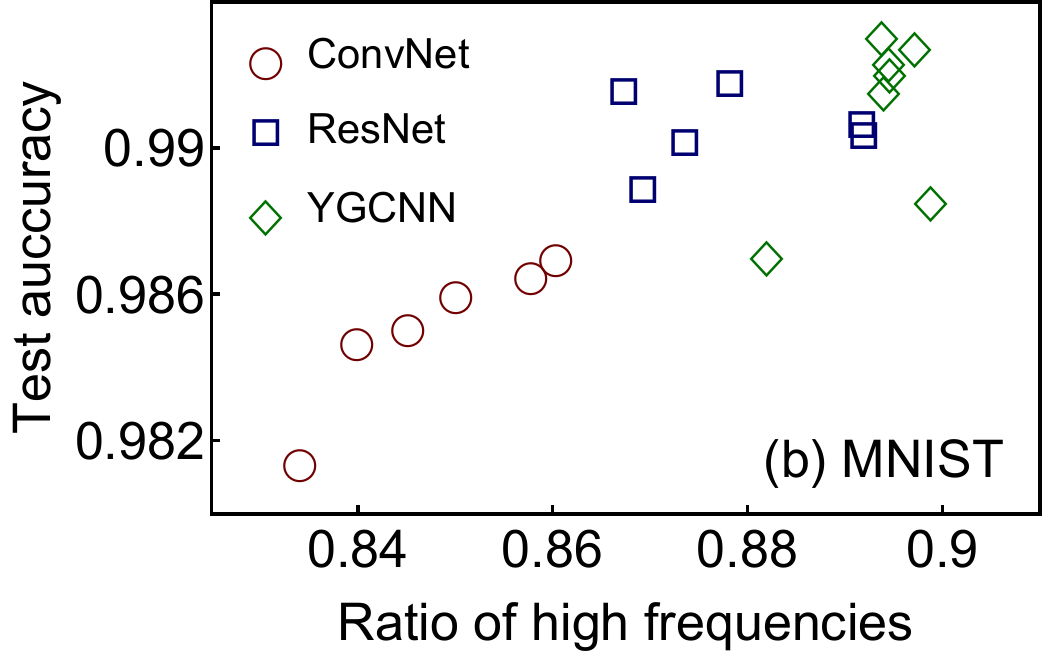}
\caption{Ratio of high frequencies is roughly proportional to the test accuracies.\label{fig:Ratio-of-high}
Ratio of high frequencies is obtained via the formula $(|\text{FFT}[\Delta_{1}]|-|\text{FFT}[\Delta_{1}]_{\text{LF}}|)/|\text{FFT}[\Delta_{1}]|$.
For Cifar-10, we turn the RGB images into gray and $|\text{FFT}[\Delta_{1}]_{\text{LF}}|$ takes the slices $[15:19,15:19]$.
For MNIST,  $|\text{FFT}[\Delta_{1}]_{\text{LF}}|$ takes the slices $[12:18,12:18]$.
The networks are trained with various epoch numbers to gain the different test accuracies. The implementation can be found in Ref. \cite{DVN/FKFJZQ_2021}.}
\end{figure}

Apart from the uncertainty principle, the results can also be understood
from the frequency-principle\cite{xu2020frequency} (F-Principle) in a straightforward way.
It is proposed by the F-Principle that “the
DNNs tend to fit training data by a low-frequency function resulting
from the smoothness/regularity of the commonly used activation functions”.
Therefore, it is harder for the neural networks to predict high-frequency
images than the low-frequency ones. To be specific, in the training
of reducing the loss function $l(f(X,\theta),Y^{*})$,
smaller values of $l$ indicate higher training (and also test) accuracies
if the network is not over fitted. For a network to distinguish among
many classes, high-frequency features are gradually resolved in
the training course. Thus, a neural network with higher accuracy contains
more high-frequency features\cite{xu2019training,wang2020high-frequency}.
In Fig. \ref{fig:Ratio-of-high}, we compare the test accuracies of
the classifiers with the proportion of the high frequencies of the
generated $\Delta_{1}$. We see that $\Delta_{1}$ contains more high
frequency components with the increasing of the test accuracies, and $\Delta_{1}$ with more
high frequencies is more difficult for a Pix2Pix network to produce.

Therefore, a more accurate classifier should generate the $\Delta_{1}$
with higher frequencies. Meanwhile, a robust classifier corresponds to
the generation (by Pix2Pix) of $\Delta_{1}$ to high precision, which is harder to achieve
if $\Delta_{1}$ contains more high frequency components. This can rationally explain the phenomenon that both TA and RA decrease with $\text{N}_{\text{epoch}}$.

% if have a single appendix:
%\appendix[Proof of the Zonklar Equations]
% or
%\appendix  % for no appendix heading
% do not use \section anymore after \appendix, only \section*
% is possibly needed

% use appendices with more than one appendix
% then use \section to start each appendix
% you must declare a \section before using any
% \subsection or using \label (\appendices by itself
% starts a section numbered zero.)
%

% Can use something like this to put references on a page
% by themselves when using endfloat and the captionsoff option.
\ifCLASSOPTIONcaptionsoff
  \newpage
\fi

% trigger a \newpage just before the given reference
% number - used to balance the columns on the last page
% adjust value as needed - may need to be readjusted if
% the document is modified later
%\IEEEtriggeratref{8}
% The "triggered" command can be changed if desired:
%\IEEEtriggercmd{\enlargethispage{-5in}}

% references section

% can use a bibliography generated by BibTeX as a .bbl file
% BibTeX documentation can be easily obtained at:
% http://mirror.ctan.org/biblio/bibtex/contrib/doc/
% The IEEEtran BibTeX style support page is at:
% http://www.michaelshell.org/tex/ieeetran/bibtex/
%\bibliographystyle{IEEEtran}
% argument is your BibTeX string definitions and bibliography database(s)
%\bibliography{IEEEabrv,../bib/paper}
%
% <OR> manually copy in the resultant .bbl file
% set second argument of \begin to the number of references
% (used to reserve space for the reference number labels box)
\bibliographystyle{IEEEtran}
\bibliography{IEEEabrv,sn-bibliography}

% biography section
%
% If you have an EPS/PDF photo (graphicx package needed) extra braces are
% needed around the contents of the optional argument to biography to prevent
% the LaTeX parser from getting confused when it sees the complicated
% \includegraphics command within an optional argument. (You could create
% your own custom macro containing the \includegraphics command to make things
% simpler here.)
%\begin{IEEEbiography}[{\includegraphics[width=1in,height=1.25in,clip,keepaspectratio]{mshell}}]{Michael Shell}
% or if you just want to reserve a space for a photo:

% You can push biographies down or up by placing
% a \vfill before or after them. The appropriate
% use of \vfill depends on what kind of text is
% on the last page and whether or not the columns
% are being equalized.

%\vfill

% Can be used to pull up biographies so that the bottom of the last one
% is flush with the other column.
%\enlargethispage{-5in}

% that's all folks
\end{document}
