# Supplementary material for: On the uncertainty principle of neural networks
Source: arXiv:2205.01493 source file (2025-01-16)
Supplement: Supplementary file 2 [file supplementary_material.pdf]

# On The Uncertainty Principle of Neural Networks: Supplementary Material

— Understanding the uncertainty principle in terms of FGSM attack

Jun-Jie Zhang, Dong-Xiao Zhang, Jian-Nan Chen, Long-Gang Pang, and Deyu Meng

## Abstract

In this supplementary material, we provide a perspective to understand the uncertainty principle of neural networks proposed in the main paper in terms of the frequency-principle. Based on the observation that an opposite direction of the FGSM attack increases both the Test Accuracy (TA) and Robust Accuracy (RA), we specifically build a pipeline named the Iterative FGSM Augmentation (IFA). In IFA, to obtain high TA and RA is equivalent to train a Pix2Pix network, which maps an image to another image, to high accuracy. Our experiments show that such an attempt to train a Pix2Pix fails at producing images containing more high frequency components. The results indicate that one can hardly expect to train a network (e.g., Pix2Pix) which resolves both the images and their conjugates to an arbitrary high accuracy simultaneously.

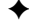

Since the Test Accuracy (TA) and Robust Accuracy (RA) of a neural network involve two procedures, it is hard to perceive the uncertainty principle directly. Thus, we provide another view to further perceive the principle.

## 1 OBSERVATION FOR OBTAINING ACCURATE AND ROBUST NETWORKS

In image classification, a well-trained neural network separates the data points (images) into several classes. If the FGSM attack decreases the classification accuracy, one will be able to attain an increase in accuracy following the opposite direction of the FGSM attack (the same phenomenon is also observed by the current literatures [1], [2]). To intuitively perceive the phenomenon, we schematically depict the effects of both the FGSM attack and its opposite in Fig. 1. The shaded areas correspond to the domains of different image classes which are determined by the loss function. The FGSM attack shifts the data points that belong to the TRUE domain towards other domains so as to attack the classification network. On the contrary, if we iteratively apply the FGSM attack in the opposite direction, we can move these data points back to their TRUE domain classes—thus inclining to gain an augmentation of the accuracies for the training set [1], [2].

To further instantiate the phenomenon, we iteratively apply the opposite FGSM attack via the formula

$$\begin{aligned} X_{n+1} &= X_n - \epsilon \cdot \text{sign}(\nabla_X l(f(X, \theta), Y^*)|_{X=X_n}) \\ &\equiv X_n + D_n, \end{aligned} \quad (1)$$

where  $X_n$  and  $X_{n+1}$  denote the images before and after the iteration. The relevant TA and RA for images  $X_{n+1}$  at different iteration steps are shown in Fig. 2, where we can see that with the increase of the iteration steps, both TA and RA show tendency of increase. Note that in order to obtain  $X_{n+1}$ , we need to evaluate the term  $\epsilon \cdot \text{sign}(\nabla_X l(f(X, \theta), Y^*)|_{X=X_n})$  which requires to pre-know the label knowledge  $Y^*$ . Hence, the opposite FGSM attack is only applicable on the training set so far.

The above phenomena is somehow inspiring. Specifically, it motivates a natural idea that if we can design similar procedures on the test set, we will increase both TA and RA simultaneously, and the deduced uncertainty principle in the paper tends to be doubtful, and we will have actually found a method to defend the adversarial attacks.

## 2 THE PIPELINE OF THE ITERATIVE FGSM AUGMENTATION

To achieve the goal, we may think of building a Pix2Pix [3], [4] network which aims to learn a mapping to directly output a proper conjugate  $\Delta_N$  from an input image  $X_0$ , where

$$\begin{aligned} \Delta_N &\equiv X_N - X_0 \\ &= X_{N-1} + D_{N-1} - X_0 = \dots = \sum_{n=0}^{N-1} D_n. \end{aligned} \quad (2)$$

- J.-J. Zhang, D.-X. Zhang and J.-N. Chen are with the Division of Computational physics and Intelligent modeling, Northwest Institute of Nuclear Technology, Shaanxi, Xi'an 710024, China  
E-mail: zjacob@mail.ustc.edu.cn
- L.-G. Pang is with the Key Laboratory of Quark & Lepton Physics of Ministry of Education, Central China Normal University, Wuhan 430079, China.
- D. Meng is with School of Mathematics and Statistics and Ministry of Education Key Lab of Intelligent Networks and Network Security, Xi'an Jiaotong University, Shaanxi, P. R. China.  
Email: dymeng@mail.xjtu.edu.cn

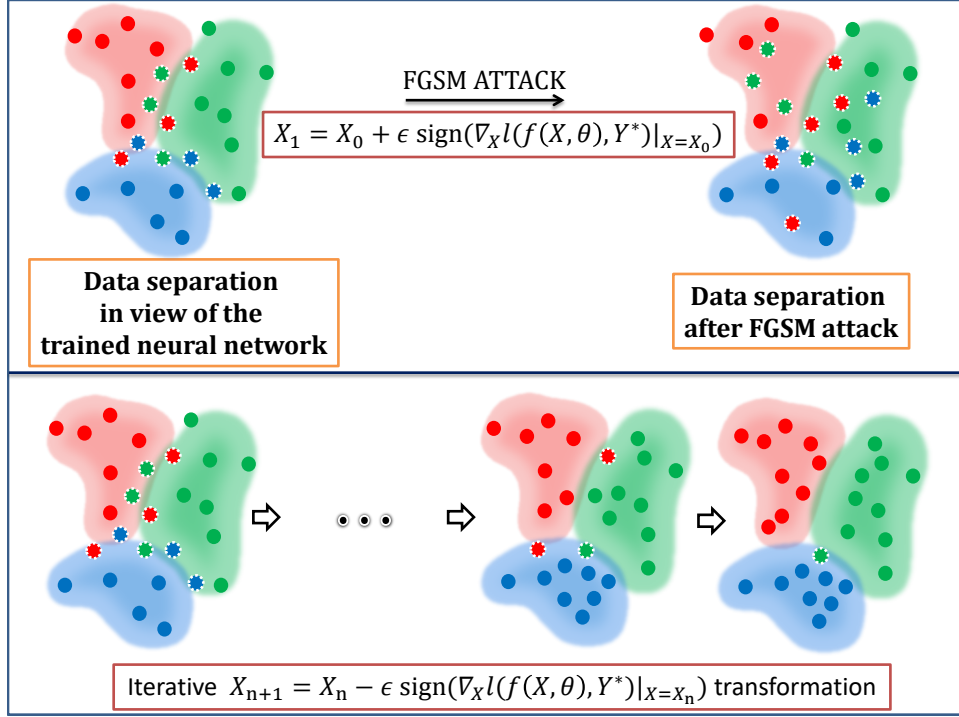

Fig. 1. Illustration of the FGSM attack and its opposite. The upper panel: FGSM attack transforms some of the images (data points) that belong to a certain domain towards other domains, leading to a decrease of the accuracy. The lower panel: the opposite direction of the FGSM attack transforms the images towards the domains with correct classification, leading to an increase of the accuracy.

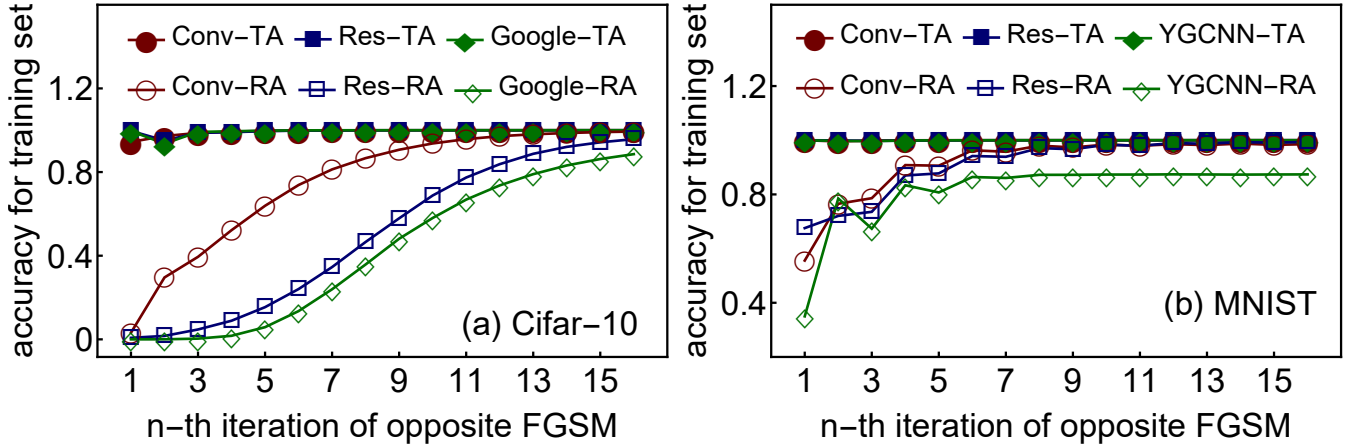

Fig. 2. Test accuracy (TA) and robust accuracy (RA) for training set. ConvNet, ResNet and GoogleNet are applied to the Cifar-10 dataset; and ConvNet, ResNet and YGCNN are applied to the MNIST dataset. The attacking strength  $\epsilon = 8/255$  and  $0.1$  for Cifar-10 and MNIST respectively. The detailed structures of these networks can be found in Ref. [3]

The capital N represents the final iteration number through Eq. (1).  $\Delta_N$  can be seen as a conjugate of the raw image  $X_0$ . With such a network, we can obtain the corresponding  $\Delta_N$  with given  $X_0$ . Once  $\Delta_N$  is obtained, we can immediately construct  $X_N$  via  $X_N = X_0 + \Delta_N$ . According to Fig. 2,  $X_N$  so obtained is expected to pose both high TA and high RA in terms of the trained classifier. We name this conjecture as Iterative FGSM Augmentation (IFA, see Fig. 3 for details). The IFA algorithm aims to connect the  $X_0$  and its conjugate  $\Delta_N$  in one single network by adopting the Pix2Pix network.

The purpose of this design is to substantiate that the Pix2Pix network cannot resolve  $X_0$  and its conjugate  $\Delta_N$  to an arbitrary high accuracy simultaneously, so as to further validate that the RA and TA cannot get sufficiently better at the same time. The uncertainty principle of neural networks can then be more faithfully verified. As will be shortly revealed, due to the uncertainty principle of neural networks, such an ideal Pix2Pix network can hardly achieve its intended purpose.

### 3 MANIFESTATION OF THE UNCERTAINTY PRINCIPLE

Now we can follow the four steps in IFA attempting to train such an ideal Pix2Pix network that generates  $\Delta_N$  providing the raw images  $X_0$ .

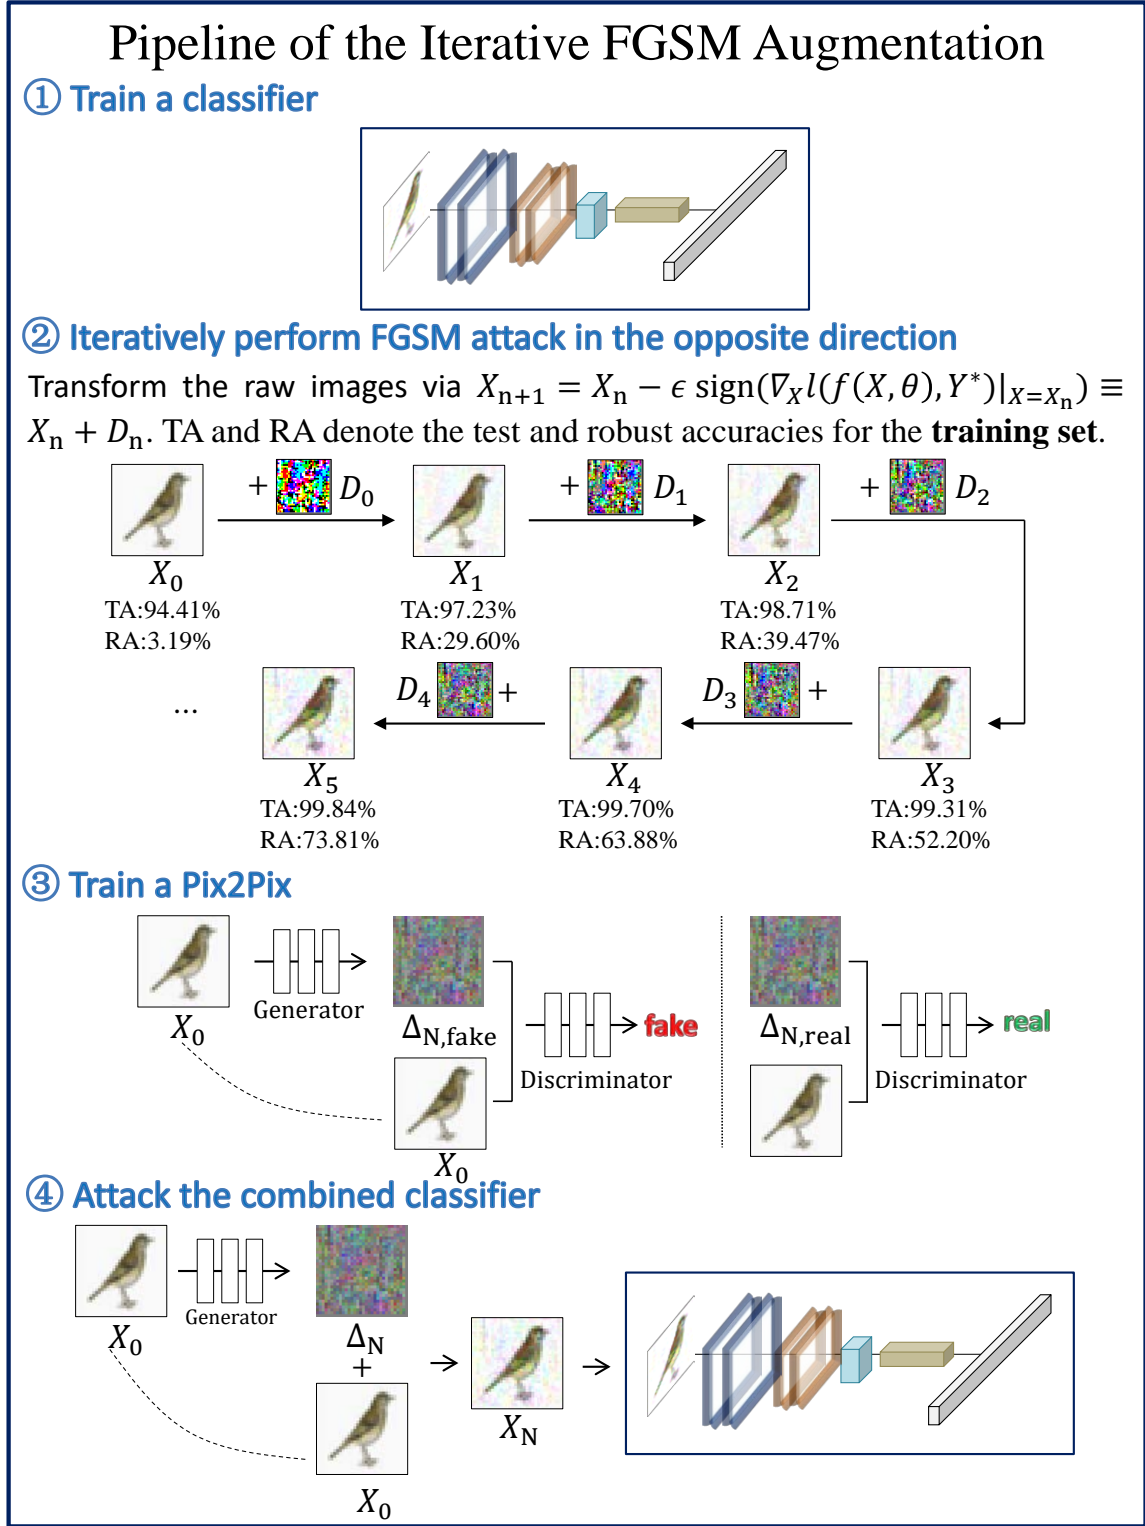

Fig. 3. The pipeline of the iterative FGSM augmentation. ① A classifier (for instance the Residual neural network) is first trained with  $N_{\text{epoch}}$  epoches, where  $X_0$  and  $Y^*$ , denote the raw images and labels. ② Based on the observation that the opposite direction of the FGSM attack increases the accuracy, we iteratively perform the FGSM attack in the opposite direction so as to increase the test accuracies (TA) and robust accuracies (RA) of the training set. Hence, as long as one obtains  $\Delta_N$  for image  $X_0$ ,  $X_0 + \Delta_N$  will have both high TA and RA. ③ For the test set, since the label  $Y^*$  is unknown,  $\Delta_N$  cannot be obtained directly. Instead, we construct a Pix2Pix network whose inputs are  $X$  and outputs are  $\Delta_N$ . ④ Providing the images  $X_0$  (in the test set) to the Pix2Pix generator, we gain its conjugation  $\Delta_N$  and  $X_N$ . Then, we evaluate the relevant TA and RA for images  $X_N$ . Note that RA is obtained via the iterative FGSM attack (with step size 4 and  $l_\infty$  loss) applied to the combined neural network (Pix2Pix+classifier).

TABLE 1

Test and robust accuries for the classifiers on MNIST dataset. CL stands for classifiers that are not combined with a Pix2Pix network and ACL stands for the classifiers Pix2Pix+Conv/Res/YGCNN.

| Network type |     | Test accuracy (%)  |       |       | Robust accuracy (%) |       |       |
|--------------|-----|--------------------|-------|-------|---------------------|-------|-------|
|              |     | $N_{\text{epoch}}$ |       |       | $N_{\text{epoch}}$  |       |       |
|              |     | 1                  | 30    | 50    | 1                   | 30    | 50    |
| ConvNet      | CL  | 97.31              | 98.71 | 98.72 | 41.44               | 50.98 | 53.74 |
|              | ACL | 99.04              | 98.87 | 99.25 | 89.53               | 93.90 | 98.00 |
| ResNet       | CL  | 98.65              | 99.50 | 99.57 | 90.88               | 98.22 | 98.27 |
|              | ACL | 99.32              | 99.15 | 89.85 | 95.44               | 52.96 | 51.03 |
| YGCNN        | CL  | 97.35              | 99.15 | 99.19 | 59.84               | 49.06 | 45.68 |
|              | ACL | 98.96              | 99.08 | 98.29 | 95.43               | 89.95 | 67.73 |

First of all, we train a few classifiers on the datasets Cifar-10 and MNIST at various epoch numbers (denoted as  $N_{\text{epoch}}$ ). In general larger  $N_{\text{epoch}}$  values correspond to more accurate classifiers. Here, we use the typical Convolutional (ConvNet), Residual (ResNet), Google (GoogleNet) networks for Cifar-10 dataset and train these networks with epoch numbers  $N_{\text{epoch}} = 1, 5, 50$ . For MNIST dataset, we use the ConvNet, ResNet, and YGCNN [5] (proposed by YASSINE GHOUZAM) networks. Since the MNIST dataset is much easier compared with the Cifar-10, TA for  $N_{\text{epoch}} = 5$  will be similar to that of  $N_{\text{epoch}} = 1$ . To observe prominent effects, the classifiers for MNIST are trained with  $N_{\text{epoch}} = 1, 30, 50$ . Once these classifiers are obtained, we can evaluate their TA and RA to see how robust the classifiers can be. For convenience, we refer the obtained TA and RA in this stage to CL, meaning the normal classifier learning (CL) without iterative FGSM augmentation.

Then we perform the second step of IFA. Since the classifiers are already trained, we can use Eqs. (1) and (2) to generate  $\Delta_N$  iteratively. The maximum iteration step is chosen to be  $N = 200$ . Generally, TA and RA for  $X_n$  will increase with the increasing of  $n$ . In step one, we have chosen three epoch numbers for each classifier. Thus, we obtain three different sets of the training weights. For example, for ConvNet on Cifar-10, we have trained weights  $\theta_{N_{\text{epoch}}=1}$ ,  $\theta_{N_{\text{epoch}}=5}$ , and  $\theta_{N_{\text{epoch}}=50}$ . For each weight, for instance  $\theta_{N_{\text{epoch}}=5}$ , we can generate  $\Delta_{200}$  using Eq. (1) and (2). This procedure can form a new dataset where  $(X_0, \Delta_{200})$  are the (input, label) pairs. At this stage, we have generated a dataset containing both the inputs  $X_0$  and the relevant conjugates  $\Delta_{200}$ .

Next, we train a Pix2Pix network with training sample pairs  $(X_0, \Delta_{200})$  following the third step of IFA. The training of Pix2Pix is an independent procedure which is irrelevant to the classifiers in step one, and does not alter the weights of the classifiers. The Pix2Pix network used here is a Generative Adversarial Network (GAN) with a U-Net structure containing 5 convolutional blocks as the encoder, and 4 deconvolutional layers as the decoder. Each convolutional block is a combination of 2 convolutional layers. The discriminator of the Pix2Pix consists of three convolutional blocks, where each convolutional block contains 1 convolutional layer with spectral normalization, 1 batch normalization layer and 1 leakyReLU layer. The specific implementation of the Pix2Pix and the classifiers can be found in Ref. [3].

Once trained, the Pix2Pix can be used to directly produce the conjugate information  $\Delta_{200}$  on the test set (the last step of IFA). With the generated  $\Delta_{200}$ , we are able to further construct images  $X_{200} = X_0 + \Delta_{200}$  and use the classifiers trained in step one to evaluate the corresponding TA and RA. Note that in the last step of IFA, we do not change the weights of the classifiers; and RA is obtained by attacking the augmented classifiers (ACL) Pix2Pix+Conv/Res/Google/YGCNN using PGD. Thus, the PGD here attacks both the Pix2Pix network and the classifiers.

In Tab. 1, we present the obtained TA and RA on MNIST dataset. From the uncertainty relation Eq. (14) in the main manuscript, we know that there exists a lower bound which is directly related to the loss function; and the values of the loss function depends on the architecture of the network and the dataset. Thus, whether one can increase TA and RA for a trained classifier simultaneously depends on both the network architecture and the dataset. The results in Tab. 1 can be interpreted in terms of two aspects:

1. If, the classifier does not reach the lower bound, it is possible for us to increase both its TA and RA, as is illustrated by the ConvNet in Tab. 1.

2. Since the test accuracy often increases with the growing epoch numbers, in some cases, the lower bound in the uncertainty relation will only be reached at relatively larger epoch numbers. Under these circumstances, one is able to increase both TA and RA at small epoch numbers while fail at larger epoch numbers. Meanwhile, the conditions for larger epoch numbers also have two folds: we cannot increase both TA and RA (the ResNet case), or we can increase RA in sacrifice of decreasing TA (the YGCNN case).

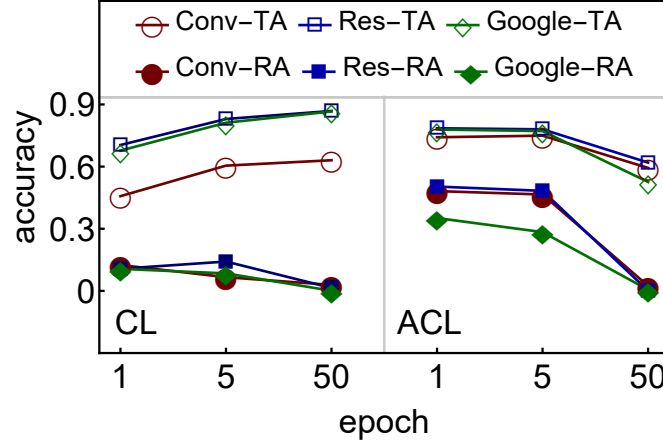

Fig. 4. Test and robust accuracies of the classifiers on Cifar-10 dataset. CL stands for classifiers that are not combined with a Pix2Pix network and ACL stands for the classifiers Pix2Pix+Conv/Res/Google. Other parameters are set the same to Fig. 2.

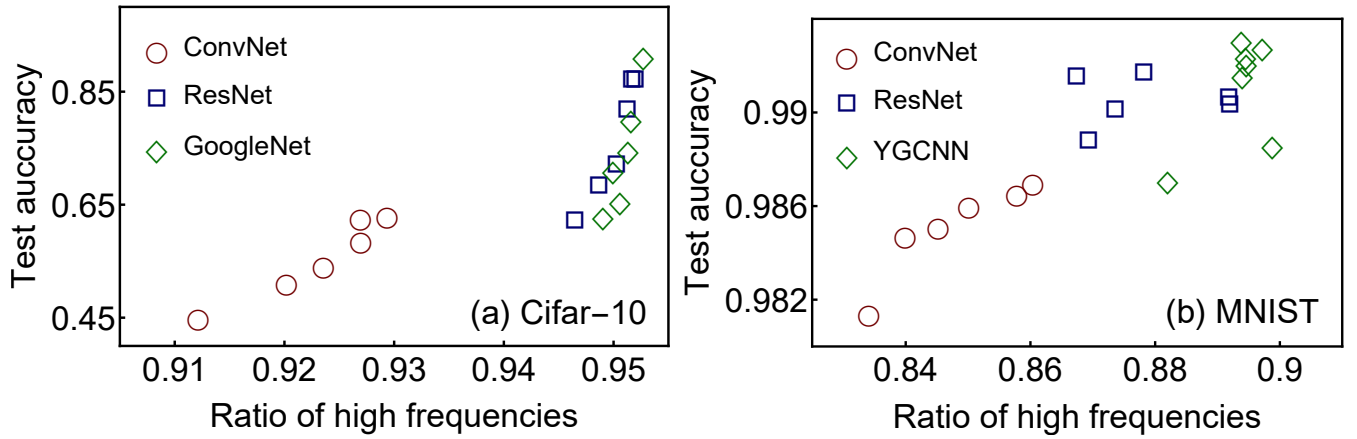

Fig. 5. Ratio of high frequencies is roughly proportional to the test accuracies. Ratio of high frequencies is obtained via the formula  $(|\text{FFT}[\Delta_1]| - |\text{FFT}[\Delta_1]_{\text{LF}}|)/|\text{FFT}[\Delta_1]|$ . For Cifar-10, we turn the RGB images into gray and  $|\text{FFT}[\Delta_1]_{\text{LF}}|$  takes the slices  $[15 : 19, 15 : 19]$ . For MNIST,  $|\text{FFT}[\Delta_1]_{\text{LF}}|$  takes the slices  $[12 : 18, 12 : 18]$ . The networks are trained with various epoch numbers to gain the different test accuracies. The implementation can be found in Ref. [3].

The similar phenomenon is also observed on Cifar-10. In Fig. 4 we give the TA and RA for classifiers ConvNet, ResNet and GoogleNet. In this scenario, an increase in TA corresponds to a decrease in RA in general, as clearly depicted in the left panel of Fig. 4, indicating that there is a trade-off between TA and RA. For the combined classifiers (Pix2Pix+Conv/Res/Google), TA and RA both decrease (Fig. 4 right panel) with the increasing of the epoch number  $N_{\text{epoch}}$ , indicating that the IFA pipeline fails at increasing TA and RA simultaneously.

In general, we see that we can hardly train a Pix2Pix network to an arbitrary high accuracy. Meanwhile, we also observe a decrease of TA and RA for ACL in some cases. This decreasing tendency manifests the difficulty for the Pix2Pix to generate ideal conjugate  $\Delta_{200}$ .

Note that the core of the IFA pipeline is that we have combined the images and their conjugates in a single network (the generator in Pix2Pix). If the uncertainty principle is not an inherent property for all neural networks, we are able to train the Pix2Pix network to arbitrary high accuracies, so that an increase of TA and RA should be observed. However, our attempt has failed so far, indicating the existence of such an uncertainty principle.

Since the Pix2Pix network directly links the inputs and the corresponding conjugates, the statement in uncertainty principle that "a neural network cannot resolve the inputs and the corresponding conjugates to arbitrary high accuracies" is now converted into "such Pix2Pix neural network cannot generate  $\Delta_N$  with given  $X$  to an arbitrary high accuracy". To this extent, we have converted a classifier into a generator, thus we state that the uncertainty principle should be a common result for general neural networks.

#### 4 THE FREQUENCY-PRINCIPLE EXPLANATION

Apart from the uncertainty principle, the results presented in Fig. 4 can also be understood from the frequency-principle [6] (F-Principle) in a straightforward way. It is proposed by the F-Principle that "the DNNs tend to fit training data by a low-frequency function resulting from the smoothness/regularity of the commonly used activation functions". Therefore,

it is harder for the neural networks to predict high-frequency images than the low-frequency ones. To be specific, in the training of reducing the loss function  $l(f(X, \theta), Y^*)$ , smaller values of  $l$  indicate higher training (and also test) accuracies if the network is not over fitted. For a network to distinguish among many classes, high-frequency features are gradually resolved in the training course. Thus, a neural network with higher accuracy contains more high-frequency features [7], [8]. In Fig. 5, we compare the test accuracies of the classifiers with the proportion of the high frequencies of the generated  $\Delta_1$ . We see that  $\Delta_1$  contains more high frequency components with the increasing of the test accuracies, and  $\Delta_1$  with more high frequencies is more difficult for a Pix2Pix network to produce.

Therefore, a more accurate classifier should generate the  $\Delta_1$  with higher frequencies. Meanwhile, a robust classifier corresponds to the generation (by Pix2Pix) of  $\Delta_1$  to high precision, which is harder to achieve if  $\Delta_1$  contains more high frequency components. This can rationally explain the phenomenon that both TA and RA decrease with  $N_{\text{epoch}}$  in Fig. 4.

## REFERENCES

- [1] J. I. Goodfellow, J. Shlens, and C. Szegedy, "Explaining and harnessing adversarial examples," in *International Conference on Learning Representations*, 2015.
- [2] A. Agarwal, R. Singh, and M. Vatsa, "The role of 'sign' and 'direction' of gradient on the performance of cnn," in *2020 IEEE/CVF Conference on Computer Vision and Pattern Recognition*, 2020, pp. 2748–2756.
- [3] J.-J. Zhang, D.-X. Zhang, J.-N. Chen, L.-G. Pang, and D. Meng, "Robust and Test accuracy of the IFA pipeline and the frequencies related," 2021. [Online]. Available: <https://doi.org/10.7910/DVN/FKFJZQ>
- [4] P. Isola, J.-Y. Zhu, T. Zhou, and A. A. Efros, "Image-to-image translation with conditional adversarial networks," in *2017 IEEE Conference on Computer Vision and Pattern Recognition (CVPR)*, 2017, pp. 5967–5976.
- [5] <https://www.kaggle.com/code/yassineghouzam/introduction-to-cnn-keras-0-997-top-6>.
- [6] J. Z.-Q. Xu, Y. Zhang, T. Luo, Y. Xiao, and Z. Ma, "Frequency principle: Fourier analysis sheds light on deep neural networks," *Communications in Computational Physics*, pp. 1746–1767, 2020.
- [7] J. Z.-Q. Xu, Y. Zhang, and Y. Xiao, "Training behavior of deep neural network in frequency domain," in *Neural Information Processing (ICONIP 2019)*, 2019, pp. 264–274.
- [8] H. Wang, X. Wu, Z. Huang, and P. E. Xing, "High-frequency component helps explain the generalization of convolutional neural networks," *2020 IEEE/CVF Conference on Computer Vision and Pattern Recognition (CVPR)*, pp. 8681–8691, 2020.
